# Supplementary material for: Experiment and model for a Stokes layer in a strongly coupled dusty plasma
Source: arXiv:2108.12482 ancillary file (2021-08-27)
Supplement: Supplementary file 1 [file SupplementalMaterial-StokesLayer.pdf]

# Supplemental Material

Experiment and model for a Stokes layer in a strongly coupled dusty plasma

J. Berumen and J. Goree

Submitted to: Phys. Rev. E June 4th, 2021

This Supplemental Material consists of this single PDF file.

Table of Contents:

I. Stokes Layer for a boundary condition that combines oscillatory and steady shear
A. Theoretical derivation 2
B. Experimental confirmation of theory 5

II. Apparatus
A. Laser intensity modulation apparatus 7
B. Camera triggering setup 9

III. Space-time diagram data for $f = 2$ Hz 11

IV. Method for determining of depth of penetration 12

# I. Stokes Layer for a boundary condition that combines oscillatory and steady shear

In this section of the Supplemental Material, we show that the solution for a Stokes Layer in a viscoelastic two-phase fluid, Eqs. (3), (22), and (24) in the main text, is also applicable if the motion of the boundary has a velocity that is a linear combination of a sinusoidal oscillation and a constant velocity. Here, equation numbers refer to the main text, unless they are prefixed by SM.

## A. Theoretical derivation

We consider a semi-infinite fluid that is viscoelastic and experiencing a drag force on a second phase. This fluid is in contact with a planar boundary at $y = 0$. This boundary can move along the $x$ axis. A semi-infinite fluid fills the space $y > 0$, and there is no slip at the boundary. As the boundary moves, momentum is transported into the fluid due to viscous diffusion, resulting in a flow that varies with space and time.

The differential equation that describes the flow within the fluid is Eq. (19) from the main text,

$$\left(1 + \tau\frac{\partial}{\partial t}\right)\left[\frac{\partial u_x}{\partial t} + \nu_g u_x\right] = \frac{\eta_0}{\rho}\frac{\partial^2 u_x}{\partial y^2}, \tag{19}$$

where $\tau$ is the Maxwell relaxation time, $\nu_g$ is the gas damping rate, $\eta_0$ is the shear viscosity of the fluid, and $\rho$ is the mass density of the fluid. We are interested only in the $x$ component of the velocity because of the symmetry of the boundary condition.

Below, we present solutions to Eq. (19) for three variations of the boundary condition. The boundary velocity is either (1) constant, (2) purely oscillatory, or (3) a combination of constant and oscillatory. The latter is our primary emphasis, because it models our experiment.

### 1. Boundary with constant velocity

For steady conditions, we set $\partial/\partial t = 0$ in Eq. (19), which is simplified to

$$\frac{\eta_0}{\rho}\frac{\partial^2 \mathcal{U}_x(y)}{\partial y^2} = \nu_g \mathcal{U}_x(y), \tag{SM1}$$

where $\mathcal{U}_x(y)$ describes the steady flow profile produced by a boundary moving at constant velocity.

Equation (SM1) has two solutions, both of them exponentials. The physical solution, which tends to zero as $y \to \infty$, is

$$\mathcal{U}_x(y) = \mathcal{U}_0 e^{-\sqrt{\frac{\rho\nu_g}{\eta_0}}y}\,, \tag{SM2}$$

where the coefficient $\mathcal{U}_0$ is the boundary's speed, which is constant.

## 2. Boundary with purely oscillatory motion (standard textbook Stokes Layer)

Here we review the theory for a Stokes Layer for a viscoelastic two-phase fluid, as we presented it in the main text.

The boundary condition is a purely oscillatory velocity for the planar surface. This boundary condition is written as Eq. (2) in the main text, which is

$$u_{b,x}(t) = \widetilde{U}\cos\omega t, \tag{2}$$

where the subscript $b$ indicates boundary.

For a boundary with a purely oscillatory motion, the solution to Eq. (19) is Eq. (3) of the main text

$$u_x(y,t) = \widetilde{U}e^{-y/\delta}\cos\left(\omega t - \frac{2\pi}{\lambda}y\right). \tag{3}$$

For a viscoelastic two-phase fluid, as given in Eq. (22) of the main text, the depth of penetration is

$$\delta_{2\mathrm{ph}} = \sqrt{\frac{2\eta_0}{\rho\omega}}\left[\frac{1}{(\chi-De)+\sqrt{(\chi-De)^2+(1+\chi De)^2}}\right]^{1/2}, \tag{22}$$

and as in Eq. (24) of the main text, the wavelength is

$$\lambda_{2\mathrm{ph}} = 2\pi\sqrt{\frac{2\eta_0}{\rho\omega}}\left[\frac{1}{-(\chi-De)+\sqrt{(\chi-De)^2+(1+\chi De)^2}}\right]^{1/2}. \tag{24}$$

We use two dimensionless variables: $De = \omega\tau$ characterizes the elasticity of the fluid, while $\chi = \nu_g/\omega$ characterizes the strength of the gas drag on the oscillatory flow.

## 3. Boundary with a combination of oscillatory motion and constant velocity

Here, we extend the above theory to a boundary condition that is generalized. In particular, the planar boundary's motion is now a combination of an oscillation $\widetilde{U}\cos\omega t$ and a constant velocity $U_0$,

$$u_{x,b}(t) = U_0 + \widetilde{U}\cos\omega t. \tag{28}$$

For this generalized boundary condition, Eq. (28) in the main text, we will show that the solution to Eq. (19), i.e., the flow profile, is

$$u_x(y,t) = U_0 e^{-\sqrt{\frac{\rho\nu_g}{\eta_0}}y} + \widetilde{U}e^{-y/\delta_{2\mathrm{ph}}}\cos\left(\omega t - \frac{2\pi}{\lambda_{2\mathrm{ph}}}y\right), \tag{31}$$

where $\delta_{2\mathrm{ph}}$ and $\lambda_{2\mathrm{ph}}$ remain the same as above, Eqs. (22) and (24) respectively.

To obtain Eq. (31), we start by separating the total flow profile $u_x(y,t)$ into a time-averaged component $U_x(y)$ and a fluctuating component $\tilde{u}_x(y,t)$

$$u_x(y,t) = U_x(y) + \tilde{u}_x(y,t). \tag{29}$$

We will find expressions separately for $U_x(y)$ and $\tilde{u}_x(y,t)$.

First, the time-averaged component $U_x(y)$ is obtained by setting $\partial/\partial t = 0$ in Eq. (19). The resulting differential equation is

$$\frac{\eta_0}{\rho}\frac{\partial^2 U_x(y)}{\partial y^2} = \nu_g U_x(y). \tag{SM3}$$

The solution of Eq. (SM3), i.e., the flow profile for the time-averaged component $U_x(y)$, is Eq. (30) in the main text

$$U_x(y) = U_0 e^{-\sqrt{\frac{\rho \nu_g}{\eta_0}}\,y}, \tag{30}$$

which is the same as Eq. (SM2) for a boundary moving with constant speed.

Next, the fluctuating component $\tilde{u}_x(y,t)$ is obtained by substituting Eqs. (29) and (30) into the differential equation, Eq. (19). After a few steps of algebra, the differential equation becomes

$$\left(1 + \tau\frac{\partial}{\partial t}\right)\left[\frac{\partial \tilde{u}_x}{\partial t} + \nu_g \tilde{u}_x\right] = \frac{\eta_0}{\rho}\frac{\partial^2 \tilde{u}_x}{\partial y^2}. \tag{SM4}$$

We note that Eq. (SM4) has the same form as Eq. (19), and it also has the same boundary condition as a Stokes Layer (an oscillation about zero). Therefore, Eq. (SM4) has the same solution, which is

$$\tilde{u}_x(y,t) = \tilde{U} e^{-y/\delta_{2\mathrm{ph}}} \cos\left(\omega t - \frac{2\pi}{\lambda_{2\mathrm{ph}}} y\right). \tag{SM5}$$

Finally, combining the two components $U_x(y) + \tilde{u}_x(y,t)$, i.e., Eqs. (30) and (SM5), we obtain the solution Eq. (31) for the generalized boundary condition.

## B. Experimental confirmation of theory

To give us confidence in our theoretical derivation above, that Eq. (31) is a solution of Eq. (19), we performed an analysis using experimental data. In particular, we verify here that the exponential time-averaged theoretical solution, Eq. (30), is obeyed reasonably well in the experiment. We do this in two different tests.

The first test, to validate the prediction made in Eq. (30), is a comparison of two experimentally obtained time-averaged flow profiles. The test is that time-averaged flow profiles, obtained two ways, should be the same. One profile is $\mathcal{U}_x(y)$, which is the profile for a run where the shear was steady. The other profile is $U_x(y)$, which is the time-average for runs with oscillatory shear. In both cases, the data are from our experiment. For the runs with oscillatory shear, we averaged the experimentally obtained velocity profiles $u_x(y,t)$ over time (for an integer number of oscillations), and since we had ten runs for each frequency we averaged over those ten runs as well.

The comparison for this first test is presented in Fig. SM1. We find that the thick curves for the time-averaged profiles $U_x(y)$ for the oscillatory runs, agree reasonably well the four profiles $\mathcal{U}_x(y)$ for the runs with steady conditions, given the noise level. The noise in the oscillatory shear run profiles can be gauged by comparing the four curves in Fig. SM1 for the four separate runs. We find this agreement not only for one frequency for the oscillatory runs, but for all three frequencies shown in Fig. SM1. This test result gives us confidence in our prediction that the time-averaged profile $U_x(y)$ for a boundary with a combined oscillatory and steady motion has the same form as the time-averaged profile $\mathcal{U}_x(y)$ for a boundary moving at constant velocity.

As the second test, we compare experiment to theory. In particular, we test whether an *e*-folding length obtained from the experiment matches one obtained from the theory.

- The experimental *e*-folding length was obtained by fitting the thick curves in Fig. SM1 to an exponential, with only one free parameter. We repeated this analysis for the three frequencies in Fig. SM1, obtaining three values for the experimental *e*-folding length in the range 1.08 – 1.28 mm. These fits were reasonably good, with an $R^2$ value mostly in the range 0.89 – 0.95. (As a verification, we also obtained the experimental *e*-folding length by fitting the thin curves in Fig. SM1 for the runs with steady shear, yielding an *e*-folding length in the range 1.03 – 1.38 mm, with an $R^2$ value in the range 0.92 – 0.99.
- The theoretical *e*-folding length is given in Eq. (30) as $[\eta_0/\rho\nu_g]^{1/2}$, which for our experimental conditions had a value 1.24 mm, calculated with an input of the values reported in the main text for $\eta_0$, $\rho$, and $\nu_g$.

The outcome of this test is that the theoretical value of 1.24 mm falls within the rage of 1.08 – 1.28 mm for the experiment. The significance of this result is that it gives us greater confidence in Eq. (30), which was used in deriving the solution Eq. (31).

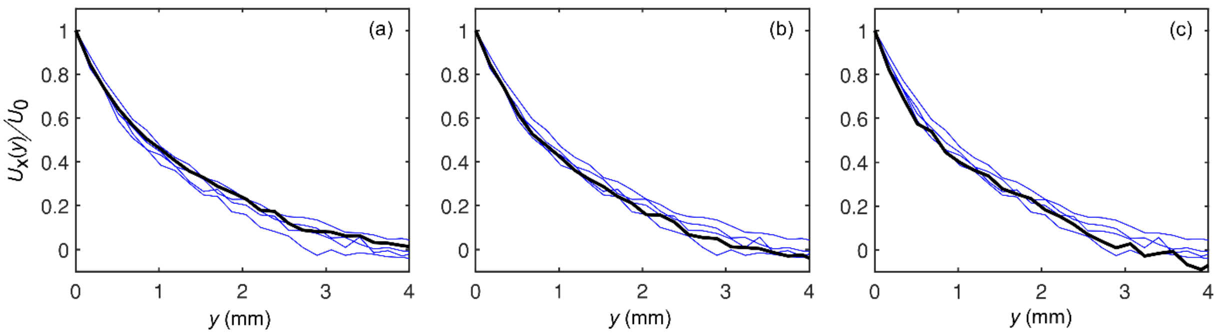


Fig. SM1. Comparison of time-averaged flow profiles from two kinds of experimental runs. For four runs done under steady shear conditions, the time-averaged profiles are shown as thin curves. For runs done with an additional oscillatory shear, we averaged the profiles for ten runs for each frequency, yielding the thick curve for (a) 0.5 Hz, (b) 1.0 Hz, and (c) 2.0 Hz. The general agreement in the shape of the two kinds of time-averaged profiles gives us confidence that the time-averaged profiles $U_x(y)$ for oscillatory shear runs can be described by Eq. (30).

# II. Apparatus

## A. Laser intensity modulation apparatus

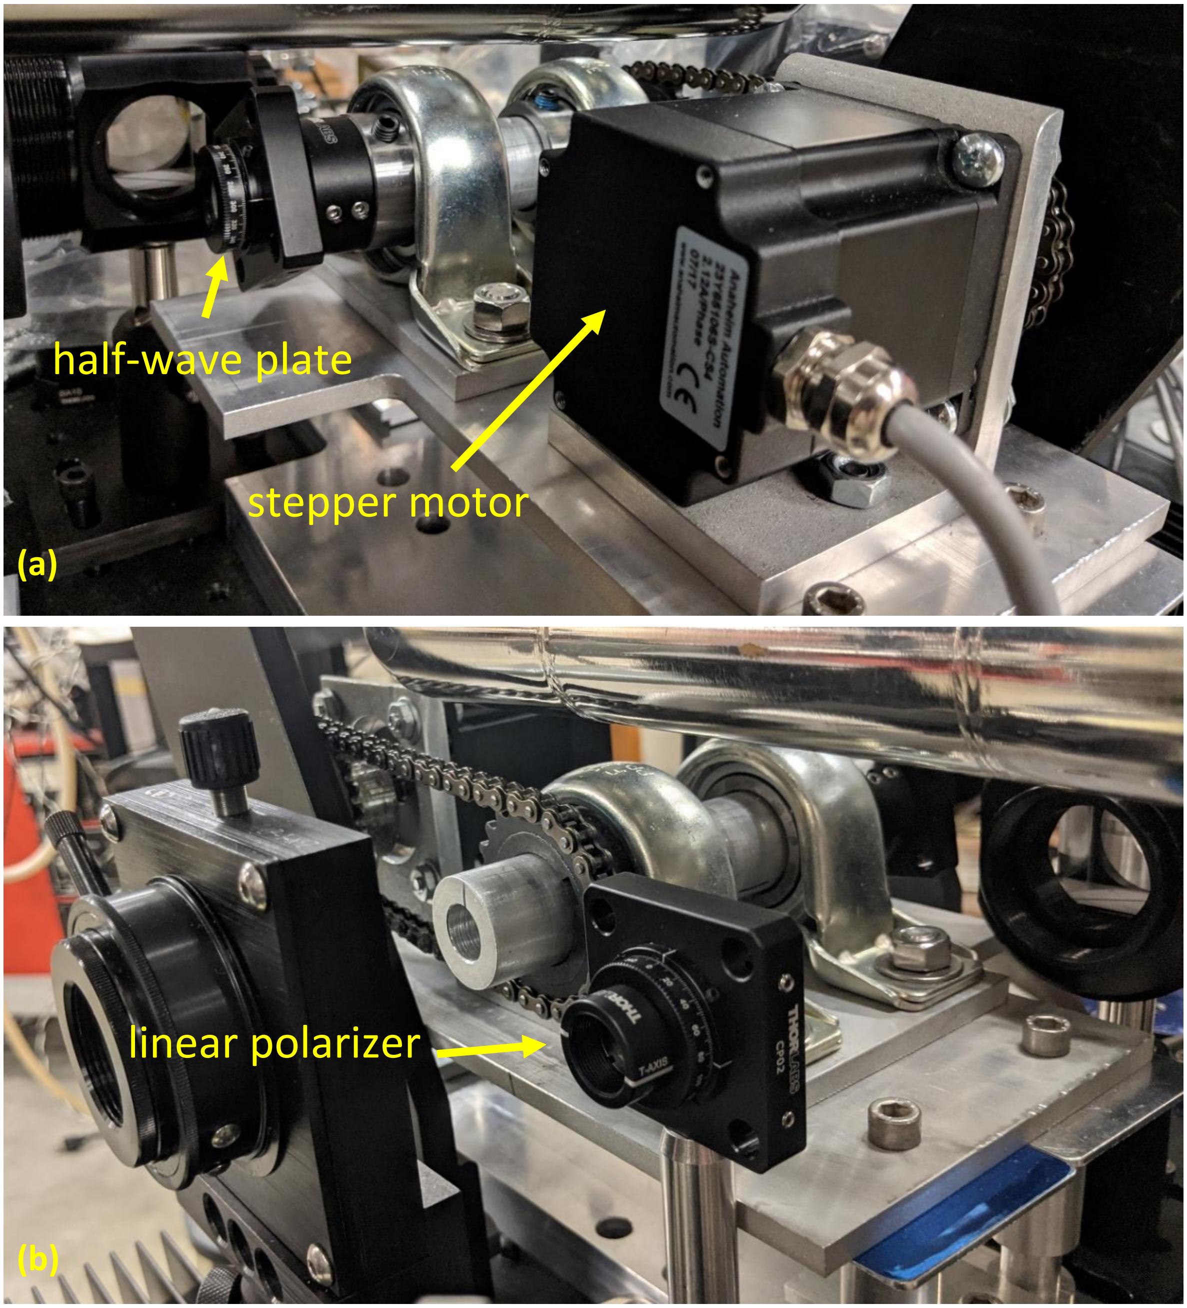


FIG. SM2. Photograph of the optical components used for modulating the intensity of the shear beam. These components are indicated in schematic form in Fig. 4 of the main text. (a) The ½-wave plate and the stepper motor are visible in this photograph. The ½-wave plate is attached to one end of a cylindrical tube. (b) The linear polarizer (P) as well as the chain and sprocket system. The motor has one sprocket, and the other sprocket is mounted on a cylinder passing through the bore of two bearings; that cylinder turns, and serves as the mount for the ½-wave plate, so that the stepper motor causes the ½-wave plate to rotate at a controlled speed.

To produce a Stokes Layer, we need to apply a localized oscillatory shear to a liquid. In our experiment, the oscillatory shear is applied onto the dust cloud (which has the properties of a liquid) using laser beams with an intensity that modulated sinusoidally. In this section of the Supplemental Material, we describe the setup used to modulate the intensity of the shear laser beam and provide photographs of the components of the setup.

Modulation of the shear beam's intensity was achieved through a combination of a rotating half-wave plate and a linear polarizer that is stationary. The entire optical system is shown in schematic form in Fig. 4 of the text. Photographs are shown here, in Fig. SM2. A ½-wave plate was attached to one end of a cylindrical tube, as shown in Fig. SM2(a), such that the plate's polarization axis was perpendicular to the path of the shear laser beam. The tube was mounted into two pillow block bearings, to minimize tilting of the wave plate as it rotated along with the tube. Tilting of the wave plate would have resulted in a spatial displacement, i.e., a misalignment of the shear laser beam.

The cylindrical tube and wave plate were rotated at a controllable frequency using a stepper motor, which was governed by a pulse generator, labelled PG2 in Fig. SM3. We used a motor with a high number of pulses per revolution to ensure a smooth rotation of the wave plate, no matter the rotation frequency. The same master clock, pulse generator PG2's internal clock, controlled two pulse generators: PG2 for the motor and PG3 for each frame of the camera recording.

## B. Camera triggering setup

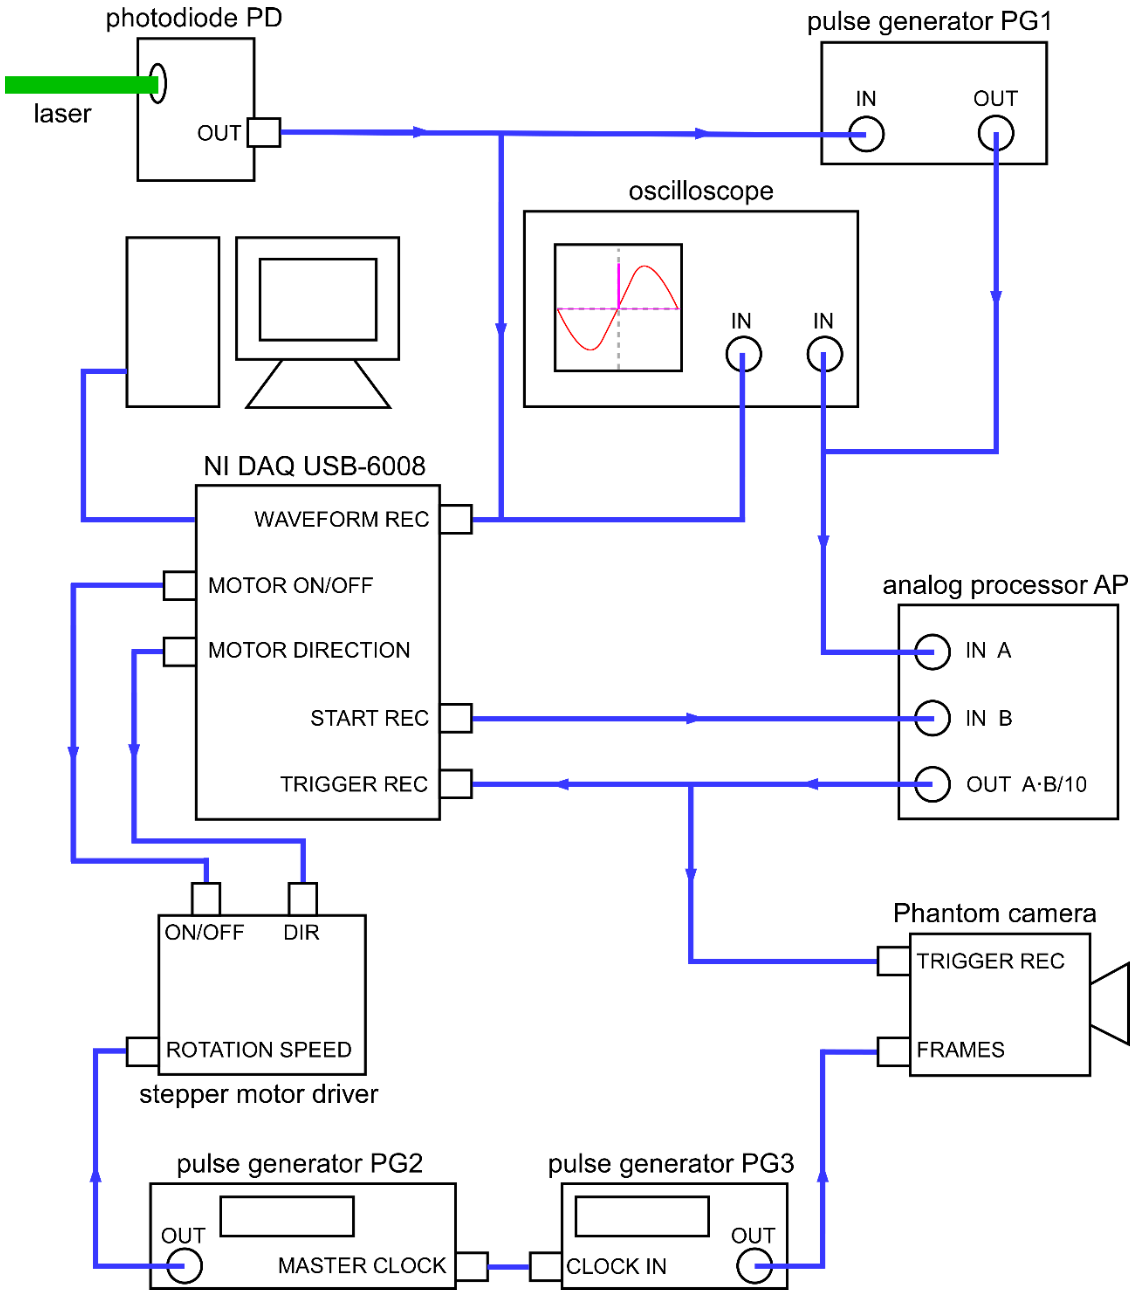


FIG. SM3. Triggering setup, which served two purposes: synchronizing the camera frame rate to be an integer multiple of the laser modulation frequency, and to start the camera recording at a consistent phase of the modulation.

In our experiment, the main diagnostic was a high-speed camera that recorded videos of the particle cloud as we applied a localized oscillatory shear. We synchronized the camera recording so that the start of each video always occurred at the same phase of the modulation cycle. In this section of the Supplemental Material, we give a brief description of the synchronization setup, which is sketched in Fig. SM3.

A photodiode detected the laser intensity as it was being modulated. The photodiode's output was used as an input for pulse generator PG1, which produced a pulse whenever the photodiode's waveform exceeded a threshold. As a result, a pulse was produced consistently at the same phase of the modulation cycle. The output of this pulse generator was applied to input A of the analog processor.

When the user expressed a desire to start the recording, the DAQ's output START REC changed from 0 V to 5 V. This output, which was otherwise steady, served as input B for the analog processor.

After START REC transitioned to 5 V, the video recording then started at the next pulse from the output of PG1. Another pulse, from the output of the analog processor, was used to trigger the camera. The function of the analog processor was to multiply its inputs A and B, and divide by 10. In our setup, input A was the output from PG1, while input B was the DAQ's output START REC. Once START REC had transitioned to 5 V, at the next pulse from PG1, the analog processor's output was a pulse, which was used to trigger both the camera recording and the recording of the photodiode's waveform by the DAQ.

## III. Space-time diagram data for $f = 2$ Hz

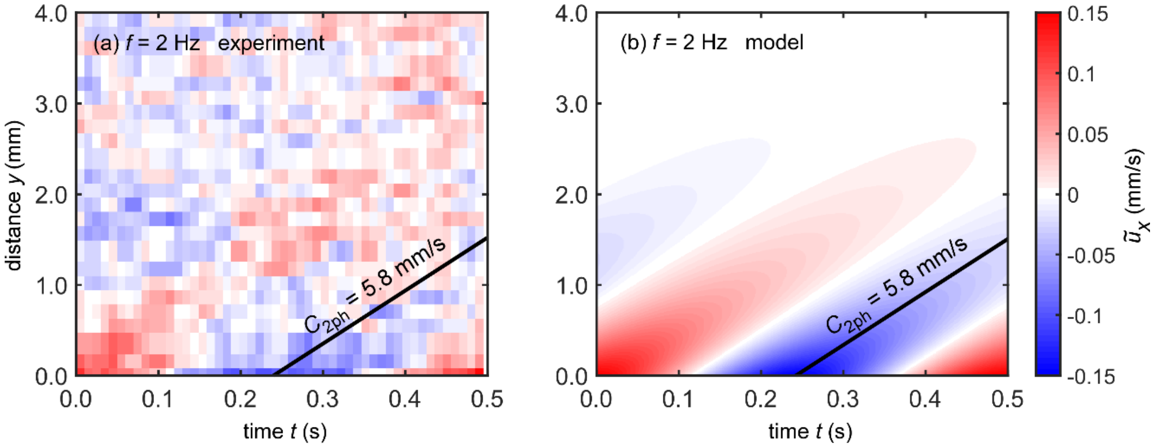


FIG. SM4. Space-time diagrams obtained from (a) experimental data and (b) our two-phase fluid model, for a modulation frequency of 2 Hz. This figure is analogous to Fig. 5 of the main text, except that it is for runs at a higher frequency for the shear laser modulation.

Here we present space-time diagrams obtained from the experiment and our two-phase fluid model, for a modulation frequency of 2 Hz. The noise level in the experiment at 2 Hz, Fig. SM4(a), is noticeably greater than at lower frequencies in Fig. 5(a) and (b) of the main text.

We believe the reason for the noisier data at high modulation frequencies was a lower flow velocity, due to two factors. First, the depth of penetration in a Stokes layer diminishes with frequency, as discussed in Sec. II of the main text. Second, due to the finite size of our dust cloud, it had a rotational inertia that tended to inhibit an overall rotation at higher frequencies

## IV. Method for determining the depth of penetration

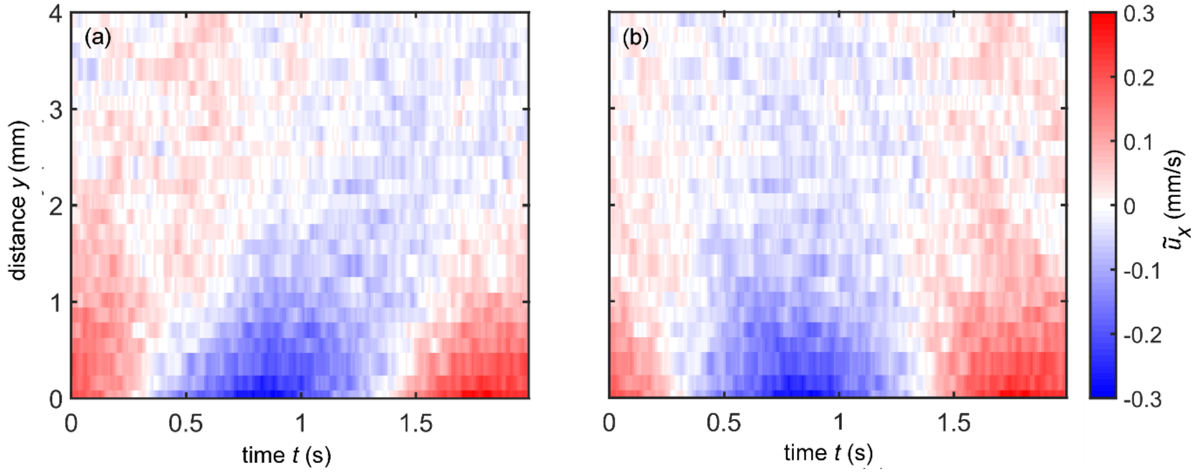


FIG. SM5. Spacetime time diagrams (a) as measured and (b) skewed. Both are for a modulation frequency of 0.5 Hz, and both have the same color bar scale for $\tilde{u}_x$.

In the main text, as part of our analysis of the experimental Stokes Layer, we provide values of the experimental depth of penetration and characteristic speed for two different modulation frequencies. In this section of the Supplemental Material, we briefly describe how we obtained those values.

As a first step, we produced a skewed version of the space-time diagram, as in Fig. SM5. The skewed diagram has the same data, but for each value of $y$ the data are shifted in time. This shift is done with a proportionality constant, so that the time shift is proportional to $y$. The value of this proportionality constant corresponds physically to a characteristic speed. We adjusted this proportionality constant until the diagram had a vertical character for the phase; this adjustment was done by a correlation method. This method generated our value for the characteristic speed $C$.

Another use for the skewed space-time diagram was to obtain the experimental value of the depth of penetration $\delta$. The data in the skewed diagram are essentially a two-dimensional array, and from this array we selected two columns corresponding to peak positive and peak negative flow velocity. These two columns of data for $\tilde{u}_x$ were fit to an exponential function, of the form $Ae^{-y/\delta}$, yielding the $e$-folding length $\delta$, which is our measured value of the depth of penetration. To obtain an error bar for $\delta$, we calculated the standard deviation from six fits, which differed in the $y$-range of data that were selected.
